# Supplementary material for: Chetaev Instability Framework for Kinetostatic Compliance-Based Protein Unfolding
Source: arXiv:2205.07375 source file (2022-05-15)
Supplement: Supplementary file 1 [file Supp.tex]

% Reset the equation counters: 
\newcounter{defcounter}
\setcounter{defcounter}{0}
\newenvironment{myequation}{%
	\addtocounter{equation}{-1}
	\refstepcounter{defcounter}
	
	\begin{equation}}
{\end{equation}}

\setcounter{figure}{0}   
%%%%%%%%%%%%%%%%%%%%%%%%%%%%%%%%%%%%%%%%%%%%%%%%%%%%%%%%%%%%%%%%%%%%%%%%%%%%%%%%%%%%%%%%%%%%%%%%%%%%%%%%%%%%%%
\section*{Supplementary Material To ``Quadratic Optimization-Based Nonlinear Control for Protein Conformation 
	Prediction''}

\noindent{\textbf{Notation.}} In these supplementary notes, we will number the equations using (s\#), the references using [S\#], and the figures using SF\#. Therefore, (s1) refers to Equation~1 in the supplementary notes while (1) refers to Equation~1 in the original article. The same holds true for the references and the figures. 

\subsection{Entropy-Loss Rate of the Protein Molecule}
There are a few equivalent ways to compute the entropy changes of a protein molecule during folding including the 
methods based on configurational entropy computations and the methods based on thermodynamics-based operational 
definitions. Here, we will use Clausius thermodynamics expression in [S1], which is similar to  
the derivations in~\cite{arkun2010prediction} in that it is based on classical thermodynamics arguments.   
Based on Clausius equation, the change of the molecule 
entropy is given by 
\begin{myequation}
\Delta S(\pmb{\theta})  = \kappa_0 \Delta \mathcal{G}(\pmb{\theta}),  
\end{myequation}
\hspace{-1.5ex} where $\kappa_0$ is a temperature-dependent constant and $\mathcal{G}(\cdot)$ is the 
aggregated free energy of the molecule given by~\eqref{eq:freePot}. Hence, 
\begin{myequation}
\frac{d}{dt} S(\pmb{\theta})  = \kappa_0 \frac{\partial \mathcal{G}}{\partial \pmb{\theta}} \dot{\pmb{\theta}} = 
\kappa_0 \frac{\partial \mathcal{G}}{\partial \pmb{\theta}} \big( 
\mathcal{J}^\top(\pmb{\theta}) \mathcal{F}(\pmb{\theta}) + \mathbf{u}_{c}\big). 
\label{eq:ineqS}
\end{myequation}
\hspace{-1.5ex} Using H\"{o}lder's and the triangle inequalities in~\eqref{eq:ineqS}, it can be seen that
\begin{myequation}
	|\dot S|  \leq  \kappa_0 \bigg|\frac{\partial \mathcal{G}}{\partial \pmb{\theta}}\bigg|_1  \bigg( 
	\big|\mathcal{J}^\top(\pmb{\theta}) \mathcal{F}(\pmb{\theta})\big|_\infty + \big|\mathbf{u}_{c}\big|_\infty\bigg). 
\end{myequation}
\hspace{-1.5ex} where $|\cdot|_1$ denotes the vector 1-norm.

\subsection{In-Depth Comparison with the Optimal Control Framework in~\cite{arkun2010prediction,arkun2011protein,arkun2012combining}}

One of the inspirations for our ODS-based control scheme for protein folding in~\eqref{eq:ODS} has been due to the pioneering work 
by Arkun and collaborators~\cite{arkun2010prediction,arkun2011protein,arkun2012combining}. Here, we provide an in-depth comparison with our work and state possible extensions of the work by Arkun and collaborators~\cite{arkun2010prediction,arkun2011protein,arkun2012combining} to our nonlinear setting.  
\begin{itemize}
	\item \textbf{Difference in the studied dynamics:} As we stated in Remark 3.1 of the article, we are considering a \emph{nonlinear dynamics} (as opposed to the \emph{linear dynamics} in~\cite{arkun2010prediction,arkun2011protein,arkun2012combining}) in the dihedral angle space of the molecule (as opposed to~\cite{arkun2010prediction,arkun2011protein,arkun2012combining}, where the state vector of the system is the Cartesian position of the $\text{C}_\alpha$ atoms). 
	
	\item \textbf{Nonlinear extension of~\cite{arkun2010prediction,arkun2011protein,arkun2012combining}:} In the linear time-invariant (LTI) setup considered by Arkun and collaborators~\cite{arkun2010prediction,arkun2011protein,arkun2012combining}, the control input is penalized  by using an infinite horizon LQR cost function to avoid extremely fast decay of excess entropy. In the context of the 
	KCM framework, a cost function in the dihedral angle space can be written similar to~\cite{arkun2010prediction,arkun2011protein,arkun2012combining} as 
	\begin{myequation}\label{eq:ArkunCost}
	J[\mathbf{u}_c] := \int_{0}^{T_f} \big( \tilde{\pmb{\theta}}(t)^\top \mathbf{Q} \tilde{\pmb{\theta}}(t)+ \rho \mathbf{u}_c(t)^\top \mathbf{P} \mathbf{u}_c(t) \big) dt, 
	\end{myequation}
	\hspace{-1.5 ex} where $\tilde{\pmb{\theta}}:= \pmb{\theta} - \pmb{\theta}^{\text{ref}}$ is the error from the current to a reference 
	conformation, e.g., the native conformation of the protein. Furthermore, the tunable parameter $\rho>0$ is employed to make a trade-off 
	between avoiding the high
	energy regions of the landscape while choosing entropically preferred 
	folding pathways by penalizing high-entropy-loss routes. \underline{The similarities with~\cite{arkun2010prediction,arkun2011protein,arkun2012combining} stop here.}  Under an LTI control setup (which is not the case for the nonlinear dynamics in~\eqref{eq:KCM_ode}) and letting $T_f \to \infty$, the solution to~\eqref{eq:ArkunCost} takes the form of the feedback control law $\mathbf{u}_c^\ast(\pmb{\theta})=-\mathbf{K}(\rho)\tilde{\pmb{\theta}}$, where the state 
	feedback gain matrix $\mathbf{K}(\rho)$ is the solution to a proper algebraic Riccati equation (ARE).  However, this ARE-based feedback control law
	is not the minimzer of the cost function in~\eqref{eq:ArkunCost} when the dynamics are governed by~\eqref{eq:KCM_ode}. \\
	\hspace{2pt} Indeed, if the system has nonlinearities, which is the case in this article, there is a need for solving a Hamilton-Jacobi equation (HJE). HJEs are partial differential equations whose explicit closed-form solutions do not exist, even in the case of a simple
	nonlinearity (see, e.g., [S3]).  \\
	\hspace{3ex} Hamilton-Jacobi equation (HJE) for the protein folding dynamics given by~\eqref{eq:KCM_ode} can obtained as follows. Let us consider the nonlinear dynamics in~\eqref{eq:KCM_ode} and the cost function in~\eqref{eq:ArkunCost}. Defining $\tilde{\pmb{\theta}}:=\pmb{\theta} - \pmb{\theta}^{\text{ref}}$,  $\tilde{\mathbf{G}}(\tilde{\pmb{\theta}}):=\mathcal{J}^\top(\tilde{\pmb{\theta}}+\pmb{\theta}^{\text{ref}})\mathcal{F}(\tilde{\pmb{\theta}}+\pmb{\theta}^{\text{ref}})$, the 
	optimal control input is given by [S4]
	\begin{myequation}
	\mathbf{u}_c^{\ast}(\tilde{\pmb{\theta}}) = -\frac{1}{2\rho} \mathbf{P}^{-1} \nabla V(\tilde{\pmb{\theta}})+
	\tilde{\mathbf{G}}(\mathbf{0}). 
	\label{eq:optimalCont}
	\end{myequation}
	\hspace{-1.5 ex} where $V(\cdot)$ is a twice continuously differentiable function that satisfies HJE 
	\begin{myequation}
	\frac{1}{4\rho} \nabla V^\top \mathbf{P}^{-1} \nabla V - ( \mathcal{J}^\top(\pmb{\theta}) \mathcal{F}(\pmb{\theta}) - \tilde{\mathbf{G}}(\mathbf{0}) ) \nabla V - \tilde{\pmb{\theta}}^\top \mathbf{Q} \tilde{\pmb{\theta}} = 0.
	\label{eq:HJE}
    \end{myequation}
	For solving the above numerically demanding partial differential equation, there are a few methods such as employing artificial
	neural networks (see, e.g., [S4]). 
	
    \item \textbf{Computational load:} Even if we neglect the complexity arising from solving HJEs in a nonlinear setting, the framework in~\cite{arkun2010prediction,arkun2011protein,arkun2012combining} requires \emph{at least twice the computational time} of our framework. This is due to the fact that the framework in~\cite{arkun2010prediction,arkun2011protein,arkun2012combining} requires knowing the final folded structure of the protein to find the proper folding pathways. Our work, on the other hand, does not require knowing this final folded structure. Rather, by following the reference vector field coming from the KCM framework, folding starts from a random structure and converges to a local minimum of the aggregate free energy of the molecule. Therefore, a fair comparison with the nonlinear extension of~\cite{arkun2010prediction,arkun2011protein,arkun2012combining} would be to run the simulations in the dihedral angle space twice; namely, finding the final folded structure $\pmb{\theta}^{\text{ref}}$ using the conventional KCM simulation in the first run, and, in the second run, using the nonlinear extension of the optimal control framework in~\cite{arkun2010prediction,arkun2011protein,arkun2012combining} (as formulated in~\eqref{eq:optimalCont},~\eqref{eq:HJE}) to guide the molecule towards the final conformation $\pmb{\theta}^{\text{ref}}$, which has been obtained from the first run.
    
    \item \textbf{The underlying philosophy of the pointwise optimal control laws:}  ODS-based  control and its resulting QP-based synthesis~\cite{spong1986control} were originally developed to address some of the challenges arising from integral performance measures such as the one in~\eqref{eq:ArkunCost}. Indeed, the QP-based synthesis avoids problems such as computationally intensive schemes and  bypassing the Pontryagin maximum principle and/or HJEs under the bound constraints on the
    allowable input torques. Even ignoring the computational complexity of such schemes, one might prefer an instantaneous or pointwise optimization procedure which optimizes the
    present state of the system without regard to future events. In the context of our QP-based control framework, the reference vector field in~\eqref{eq:KCM_vecField} guides the protein towards its native conformation on the folding landscape. 
\end{itemize}

\subsection{Proof of Proposition~\ref{prop:LipCont}}

\begin{proof}
	The solution $\omega$ to the linear programming problem  
	in~\eqref{eq:unique} is the width of a feasible set associated with the QP in~\eqref{eq:ODS}. Furthermore, Lipschitz continuity of $ \mathcal{J}^\top(\pmb{\theta}) \mathcal{F}(\pmb{\theta})$  at conformation $\pmb{\theta}_0$ implies Lipschitz continuity of $\mathbf{G}(\pmb{\theta})$ in the QP. Following Theorem~1 in~[S5], which is based on Mangasarian-Fromovitz regularity conditions~[S6], uniqueness and Lipschitz continuity of the control input follow. 
\end{proof}

\subsection{Proof of Proposition~\ref{prop:trajRel}}
\begin{proof}
	Employing the control input~\eqref{eq:KCM_control} in~\eqref{eq:KCM_ode} and noting that the iteration in~\eqref{eq:KCM_alg} is the forward Euler difference equation for the closed-loop dynamics with time step $h$, the rest of the proof
	follows a standard argument from numerical analysis (see, e.g., the proof of Theorem 1.1 in~[S7]).
\end{proof}
\subsection{Details of Implementation and Computational Complexity of the Overall Algorithm}

\noindent\textbf{Details of implementation.} A flowchart of the program is depicted in Figure~\ref{fig:flowChart}. The convergence 
criteria, following PROTOFOLD~I~\cite{kazerounian2005protofold}, is that the magnitude of all of the joint equivalent torques to be less 
than or equal to 1 kcal/(mol.A), which is in accordance with the experimentally determined values in folded proteins. Our QP-based control input generation block is using the MATLAB `\texttt{quadprog}' routine, where we are using the `\texttt{interior-point-convex}' as the QP numerical solver. After performing the direct kinematics calculations on the chain, we are using the `\texttt{molecule3D}' program [S9] for drawing the protein molecules. Interested readers are encouraged to contact the corresponding author (email:\texttt{amohmmad@umich.edu}) for obtaining a copy of the program.

\noindent\textbf{Computational complexity.} The big O notation for complexity analysis of numerical 
algorithms can be defined as follows. Given two real-valued functions $f(\cdot)$ and $g(\cdot)$, we say 
that $f(x)=\mathcal{O}(g(x))$ if there exists a positive real number $M$ and a real number $x_0$ such that 
$|f(x)|\leq M |g(x)|$ for all $x\geq x_0$. 

The QP given by~\eqref{eq:ODS} belongs to the class of box-constrained convex  quadratic programs that can be efficiently solved using  interior-point algorithms (see, e.g., [S8]). The time needed for solving such a QP using interior-point methods is of order $\mathcal{O}(N^3)$, where there are $N-1$ peptide planes in the protein molecule. Furthermore, if there are $N_a$ atoms in the chain, the computational complexity associated with computing the intramolecular forces at each iteration is of order $\mathcal{O}(N_a^2)$. Finally, the computational complexity associated with direct kinematics calculations is of order $\mathcal{O}(N)$. 
\begin{figure}[t]
	\centering
	\includegraphics[width=0.52\textwidth]{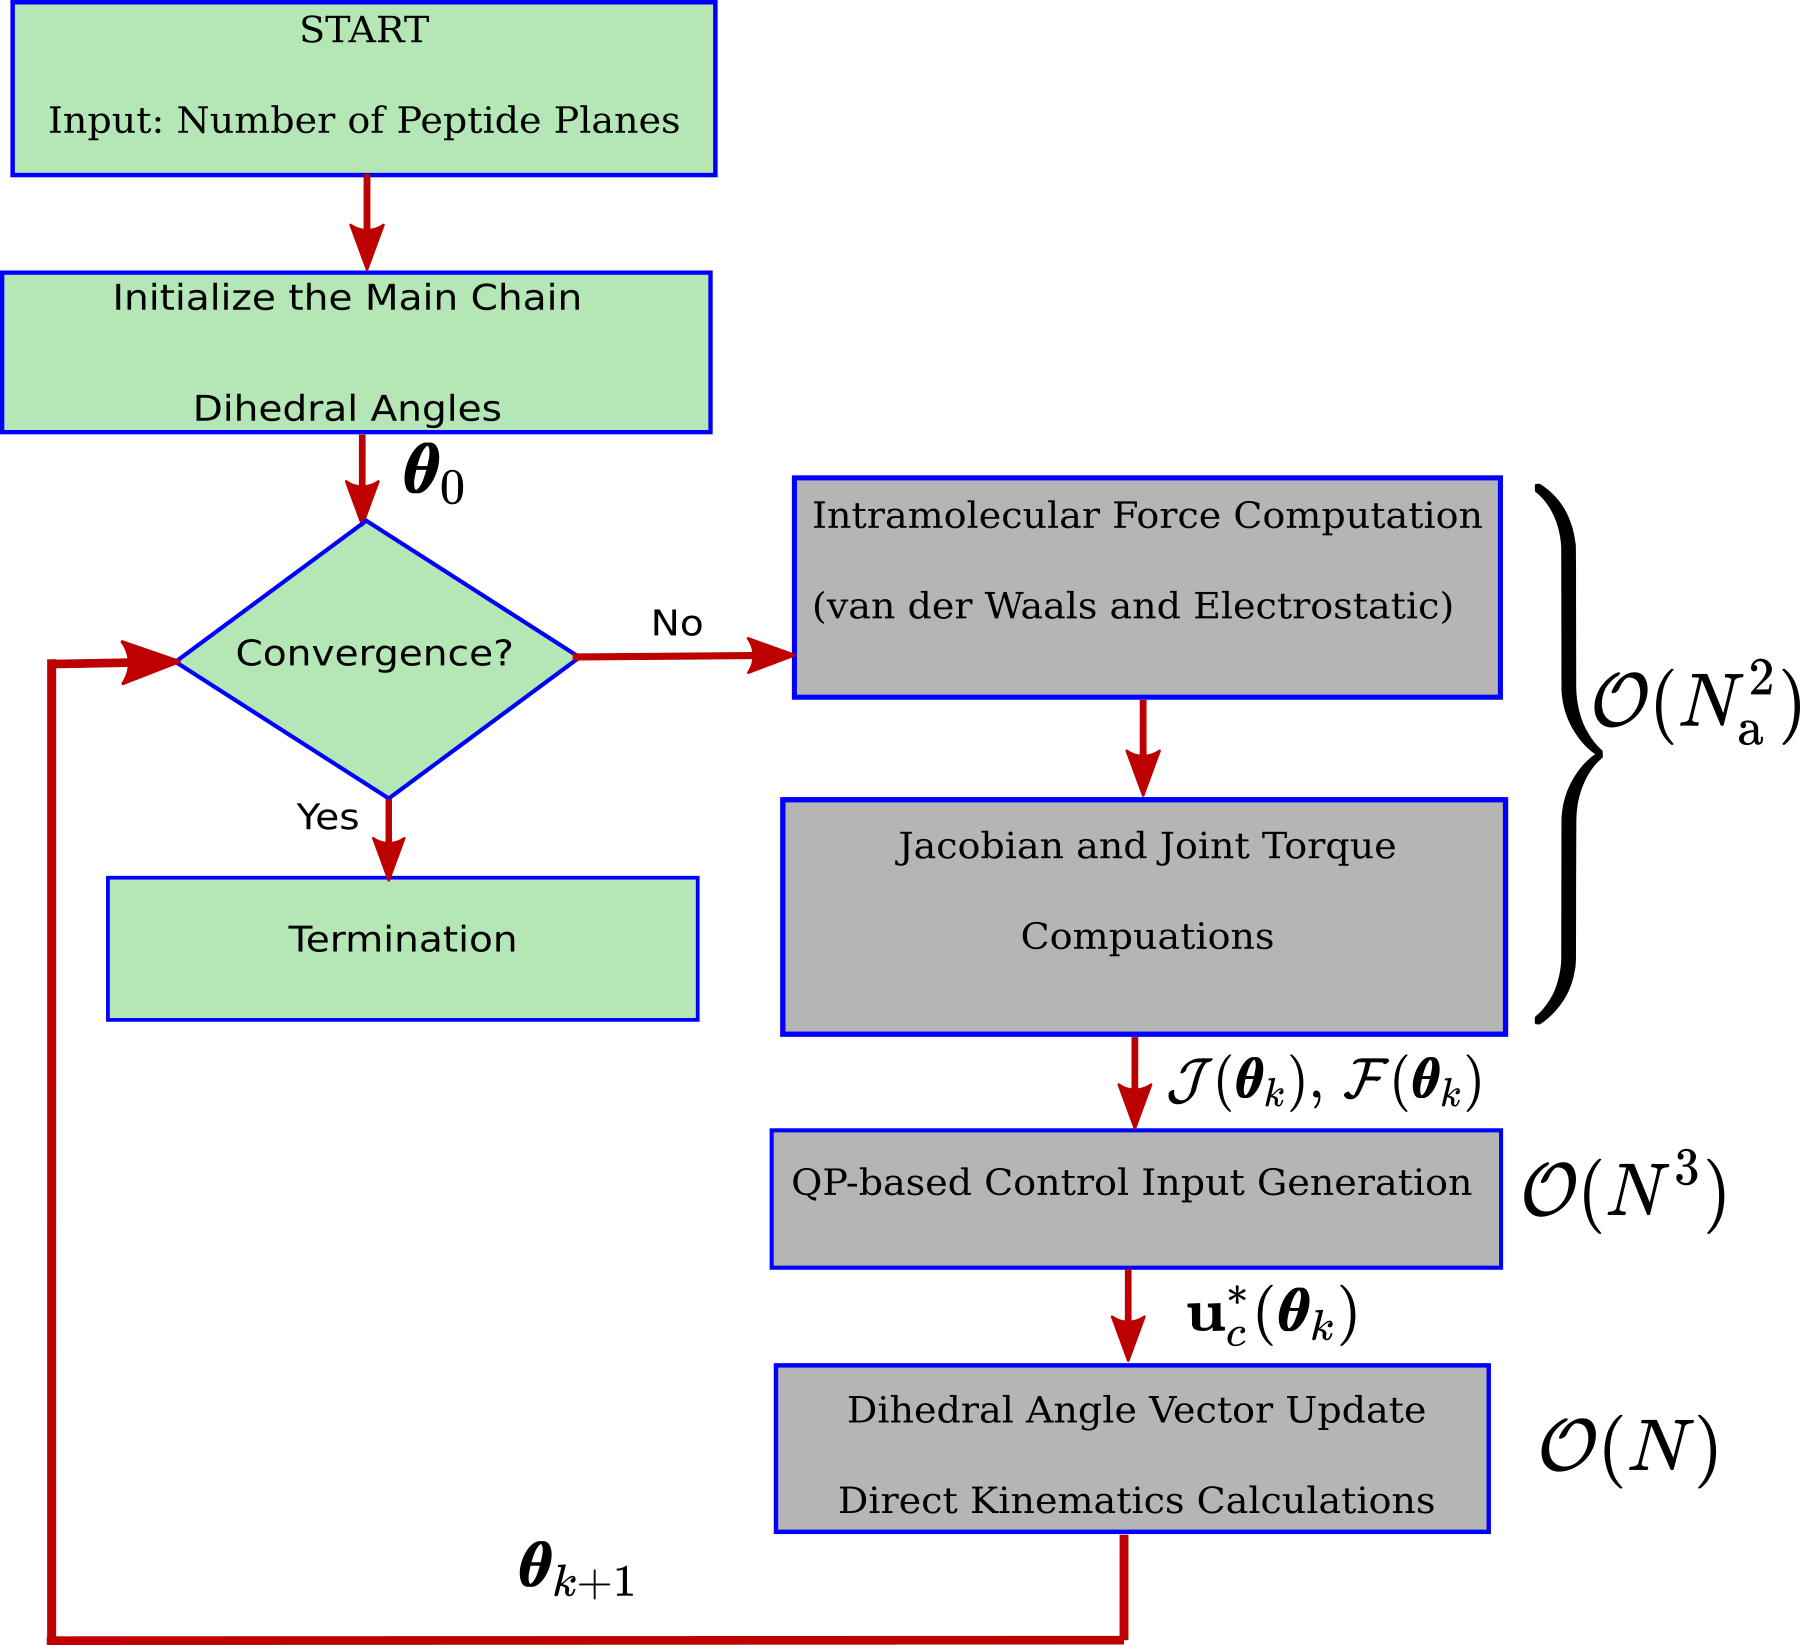}
	\caption{\small The flowchart of the computer program. Contact the corresponding author 
		(email:\texttt{amohmmad@umich.edu}) for obtaining a copy of the program.}
	\vspace{-1.5ex}
	\label{fig:flowChart}
\end{figure}

\noindent\textbf{Initial conformation of the protein molecule.} In the presented simulation results in 
the paper, the initial protein conformation  vector (in degrees) is given by 
\begin{align}
\nonumber
\pmb{\theta}_0 =  \big[ & 28.3, 28.6, 26.1, 28.7, 27.7, 26.0, 26.6, 27.5, 28.8, \cdots \\
\nonumber
& 28.8,  26.2,  28.8, 28.8, 27.2, 28.3, 26.2, 27.1, 28.7, \cdots \\
\nonumber
& 28.3, 28.8, 27.8, 25.8\big]^{\circ\top}.
\end{align}
\begin{figure*}[t]
	\centering
	\includegraphics[width=0.65\textwidth]{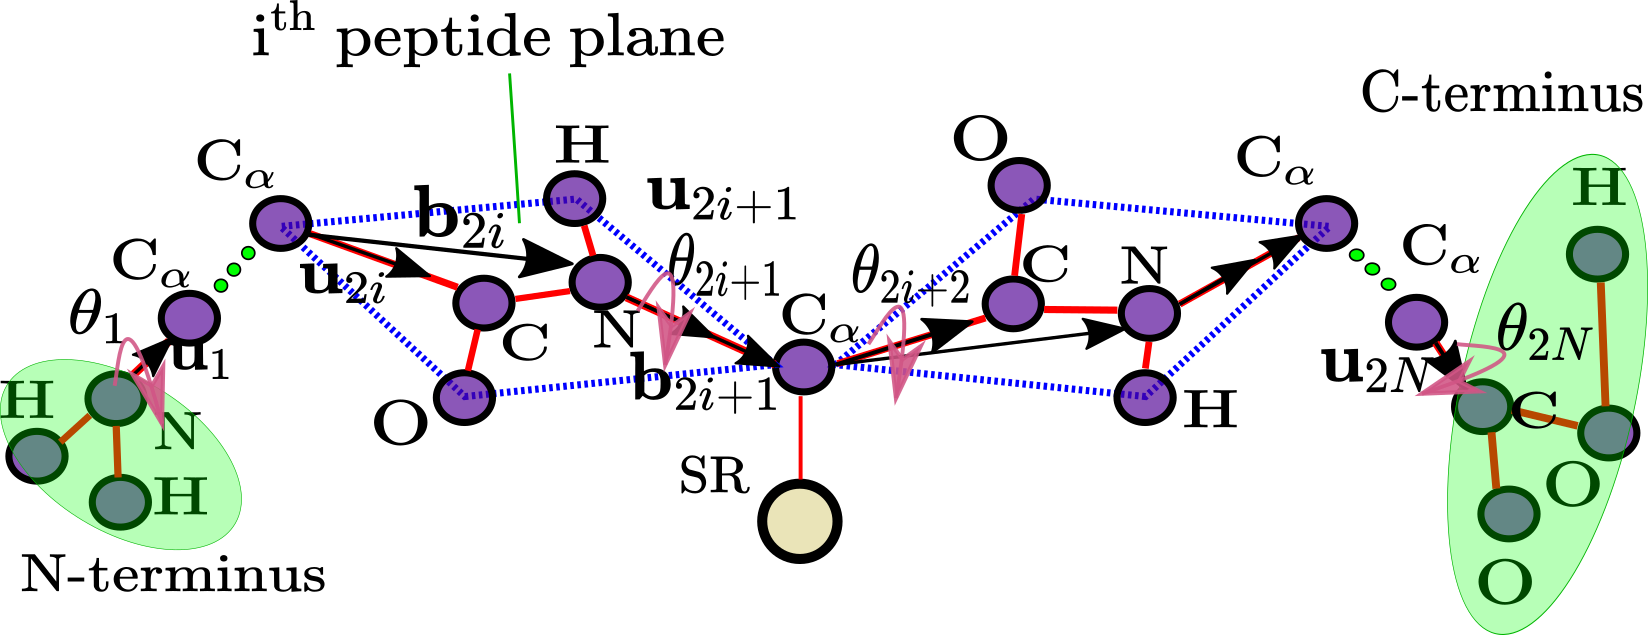}
	\caption{\small The protein molecule kinematic structure under the 
		$\text{C}_\alpha-\text{CO}-\text{NH}-\text{C}_\alpha$ coplanarity assumption.}
	\vspace{-1.5ex}
	\label{fig:protBasic1}
\end{figure*}

\section*{Supplementary References}
\small{
\noindent [S1]\hspace{1pt} S. Hikiri, T. Yoshidome, and M. Ikeguchi. ``Computational methods for configurational entropy using internal and Cartesian coordinates,'' \emph{J. Chem. Theory Comput.}, vol. 12, no. 12, pp. 5990-6000, 2016.\\

\noindent [S2]\hspace{1pt} T. Ohtsuka. ``Solutions to the Hamilton-Jacobi equation with algebraic gradients,'' \emph{IEEE Trans. Automat. Contr.}, 56(8), pp. 1874-1885, 2010.\\

\noindent [S3]\hspace{1pt} C-H. Won, S. Biswas. ``Optimal control using an algebraic method for control-affine non-linear systems,'' Int. J. Contr., vol. 80, no. 9, pp. 1491-1502, 2007.\\

\noindent [S4]\hspace{1pt} T. Cheng, F. L. Lewis and M. Abu-Khalaf. ``Fixed-final-time-constrained optimal control of nonlinear systems using neural network HJB approach,'' \emph{IEEE Trans. Neural Netw.}, vol. 18, no. 6, pp.1725-1737, 2007.\\

\noindent [S5]\hspace{1pt} B. Morris, M. J. Powell, and A. D. Ames. ``Sufficient conditions for the Lipschitz continuity of QP-based multi-objective control of humanoid robots,'' in \emph{Proc. 52nd IEEE Conf. Dec. Contr.}, Firenze, Italy, Dec. 2013, pp. 2920-2926.\\

\noindent [S6]\hspace{1pt} O. L., Mangasarian, and S. Fromovitz. ``The Fritz John necessary optimality conditions in the presence of equality and inequality constraints,'' J. Math. Anal. Appl., vol. 17, no. 1, pp. 37-47,  1967.\\

\noindent [S7]\hspace{1pt}  A. Iserles, \emph{A first course in the numerical analysis of differential
	equations}. Cambridge University Press, 2009, no. 44.\\

\noindent [S8]\hspace{1pt} Y. Wang,  and S. Boyd.  ``Fast evaluation of quadratic control-Lyapunov policy,'' IEEE Trans. Contr. Syst. Technol., vol. 19, no. 4, pp. 939-946, 2010.\\

\noindent [S9]\hspace{1pt}  A. Ludwig. \emph{molecule3D} (2016). Accessed: Oct. 2020. [Online]. Available: https://www.mathworks.com/matlabcentral/fileexchange/55231-molecule3d, MATLAB Central File Exchange. 
}
